# Supplementary material for: Large Spectral Density Matrix Estimation by Thresholding
Source: arXiv:1812.00532 source file (2018-12-03)
Supplement: Supplementary file 1 [file appendix_proof_for_main_results.tex]

\section{Extra Proof of Main Results}

\subsection{Proof for Lemma \ref{lemma: hason_bound_time_gauss}}
\begin{proof}
we can write $vec(\mathcal{\mathcal{X}}^\top)\stackrel{d}{=}\Sigma^{1/2}Z$, where $\Sigma$ is the covariance matrix of $vec(\mathcal{\mathcal{X}}^\top)$ and $Z\sim N(0,I)$. Then based on Hanson-Wright inequality \citep{rudelson2013hanson}, there exists a universal constant $c>0$ such that 

\begin{equation}
\label{eq: hanson1}
\begin{aligned}
&\mathbb{P}\left(\left|vec(\mathcal{\mathcal{X}}^\top)^\top A ~vec(\mathcal{\mathcal{X}}^\top) - \mathbb{E} \left[vec(\mathcal{\mathcal{X}}^\top)^\top A~ vec(\mathcal{\mathcal{X}}^\top)~\right]\right| >2\pi\eta\vertiii{f}\right) \\
&= \mathbb{P}\left(\left|Z^\top \Sigma^{1/2}A\Sigma^{1/2}Z - \mathbb{E}\left[ Z^\top \Sigma^{1/2}A\Sigma^{1/2}Z \right]\right|>2\pi \eta\vertiii{f}\right)\\
&\le 2\exp\left(-c\min\left(\cfrac{2\pi \eta\vertiii{f}}{\|\Sigma^{1/2}A\Sigma^{1/2}\|},\cfrac{4\pi^2\eta^2\vertiii{f}^2}{\|\Sigma^{1/2}A\Sigma^{1/2}\|_F^2}\right)\right).
\end{aligned}
\end{equation}

With lemma \ref{lemma:max-L2-norm}, $\|\Sigma^{1/2}A\Sigma^{1/2}\|\le \|\Sigma\|\|A\|\le 2\pi \vertiii{f} \|A\|$. It follows from \citet{golub2012matrix},

\begin{equation}
\begin{aligned}
&\|\Sigma^{1/2}A\Sigma^{1/2}\|_F \le \sqrt{\rank(\Sigma^{1/2}A\Sigma^{1/2})} \|\Sigma^{1/2}A\Sigma^{1/2}\|\\
&\le \sqrt{\rank(A)} \|\Sigma^{1/2}A\Sigma^{1/2}\| \le 2\pi \sqrt{\rank(A)} \|A\|_2^2 \vertiii{f}.
\end{aligned}
\end{equation}
Then plugging in the bounds for $\|\Sigma^{1/2}A\Sigma^{1/2}\|$ and 
$\|\Sigma^{1/2}A\Sigma^{1/2}\|_F$ into \eqref{eq: hanson1} completes the proof.
\end{proof}

\subsection*{Proof for lemma \ref{prop:order_Bias}}
\begin{proof}
We will prove the lemma on by on for its three conditions. Proof for all three conditions use one simple fact that 
\begin{equation}
\sum_{\ell=1}^n \ell x^\ell = \frac{x(1+nx^{n+1}-(n+1)x^n)}{(1-x)^2}.
\end{equation}

\parapgrapg{Condition 1}: Directly plug the bound on $|\Gamma(\ell)|_{\infty, \infty}$ and with $|\Gamma_{r,s}(\ell)|\le \|\Gamma(\ell)\|_{\infty, \infty}$, we have 

\begin{equation}
\Omega_n \le \sum_{\ell=1}^n \ell \|\Gamma(\ell)\|_{\infty, \infty}\le  2\sum_{\ell=1}^n \ell \rho^{\ell} = \frac{2\rho(1+n\rho^{n+1}-(n+1)\rho^n)}{(1-\rho)^2}.
\end{equation}

For $L_n$, 
\begin{equation}
L_n \le 2\sum_{\ell> n} \|\Gamma_{\ell}\|_{\infty, \infty} \le 2\sum_{\ell>n} \rho^\ell = \frac{2\rho^{n+1}}{1-\rho}. 
\end{equation}

\paragraph{condition 2}: We show $\rho$ mixing condition leads to condition 1 as 
\begin{equation}
\begin{aligned}
\Gamma_{rs}(\ell) &= \frac{e_r^\prime X_{\ell}X_{0}^\top e_s}{\sqrt{|\Gamma_{rr}(0)||\Gamma_{ss}(0)|}}\sqrt{|\Gamma_{rr}(0)||\Gamma_{ss}(0)|}\\
& \le c_1 \|\Gamma(0)\|_{\infty, \infty} \exp(-c_2\ell).
\end{aligned}
\end{equation}
Then take first constant in condition 1 as $c_1 \|\Gamma(0)\|_{\infty, \infty}$ and the second constant in condition 1 as $\exp(-c_2)$, we finish the proof.

\paragraph{Condition 3}: Consider the infinite moving average representation of $\tilde{X}_t$ 
\begin{equation}
\tilde{X}_t = \sum_{\ell=0}^\infty \tilde{B}_\ell \varepsilon_{t-\ell}, 
\end{equation}
where $\tilde{B}_\ell = (\tilde{A}_1)^\ell$ and autocovariance becomes
\begin{equation}
\Gamma(\ell) = \sum_{t=0}^\infty \tilde{B}_{t} \begin{bmatrix}
I_{p} & \mathbf{0} &\ldots & \mathbf{0} \\
\mathbf{0} &  \mathbf{0} & \ldots & \mathbf{0} \\
\vdots  & \ddots  &  \mathbf{0} & \mathbf{0} \\
\mathbf{0} &\ldots   &  \mathbf{0} & \mathbf{0}
\end{bmatrix}
\tilde{B}_{t+\ell}^\top. 
\end{equation}

Considering 
\begin{equation}
\|\tilde{A}^\ell\| = \|SD^\ell S^{-1}\| = \kappa(p)\rho(\tilde{A}_1)^\ell, 
\end{equation}
\begin{equation}
\label{eq:}
\begin{aligned}
\|\Gamma(\ell)\| &\le  \sum_{t=0}^\infty  \|\tilde{B}_{t}\|\|\tilde{B}_{t+\ell}\|\\
&\le \kappa(p) \sum_{k=\ell}^{\infty} \rho^k(\tilde{A}_1) = \kappa(p)\frac{\rho^\ell(\tilde{A}_1)}{1-\rho(\tilde{A}_1)}.
\end{aligned}
\end{equation}
Then noticing $\|\Gamma(\ell)\|_{\infty,\infty}\le \|\Gamma(\ell)\|$, using \eqref{eq:l-gamma-l-sum}
\begin{equation}
\begin{aligned}
\Omega_n &\le 2\sum_{\ell=1}^n |\ell|\|\Gamma(\ell)\| \\
&\le 2\kappa(p) \sum_{\ell=1}^n \ell \frac{\rho(\tilde{A}_1)^\ell}{1-\rho(\tilde{A}_1)} = 2\kappa(p)\frac{\rho(\tilde{A}_1)(1+n\rho^{n+1}(\tilde{A}_1)-(n+1)\rho(\tilde{A}_1))}{(1-\rho(\tilde{A}_1))^3}.
\end{aligned}
\end{equation}

For $L_n$, 
\begin{equation}
L_n \le 2\sum_{\ell\ge n} \|\Gamma(\ell)\| = 2\kappa(p)\sum_{\ell \ge n}\frac{\rho^\ell(\tilde{A}_1)}{1-\rho(\tilde{A}_1)} = 2\kappa(p)\frac{\rho^{\ell}(\tilde{A})}{(1-\rho(\tilde{A}_1))^2}.
\end{equation}
\end{proof}

\subsection{Proof for Proposition \ref{prop:bias_bound}}
\begin{proof}
It suffices to show that for any unit vector $e_r,e_s$, 
\begin{equation}
\begin{aligned}
\left|e_r^\top \left[\mathbb{E}\hat{f}(\omega_j) - f(\omega_j)\right]e_s\right| \le \frac{m}{n}\Omega_n(f_X) + \frac{1}{2\pi}\left(\frac{\Omega_n(f_X)}{n}+L_n(f_X)\right). 
\end{aligned}
\end{equation}
Recall 
\begin{equation}
\hat{f}(\omega_j) = \frac{1}{2\pi}\frac{1}{2m+1} \sum_{\ell =-m}^m I(\omega_{j+\ell}), 
\end{equation}
we could have 
\begin{equation}
\label{eq:mul_dev}
\begin{aligned}
&\left|e_r^\top \left[\mathbb{E}\hat{f}(\omega_j) - f(\omega_j)\right]e_s\right| 
\le \left|e_r^\top \left[\frac{1}{2\pi}\mathbb{E}I(\omega_j) - f(\omega_j)\right]e_s\right|\\
&+\frac{1}{2\pi(2m+1)} \sum_{\ell = -m}^m |e_r^\top\left[\mathbb{E}I(\omega_{j+\ell}) - I(\omega_{j})\right]e_s|.
\end{aligned}
\end{equation}
With definition of $I_n(\omega_j)$ in \eqref{eq:single_periodogram}, we have 
\begin{equation}
\label{eq:mul_dev1}
\begin{aligned}
\left|\frac{1}{2\pi} e_r^\top \left[\mathbb{E} I(\omega_j) - 2\pi f(\omega_j)\right]e_s\right| &= \frac{1}{2\pi}\left|\sum_{|k|\le n} \frac{k}{n}  (\Gamma_{rs}(k)) e^{-i\omega_j k}+\sum_{|k|>n} (\Gamma_{rs}(k)) e^{-i\omega_jk}\right|\\
&\le \frac{1}{2\pi} \left [\sum_{|k|\le n} \frac{k}{n}  |\Gamma_{rs}(k)|+ \sum_{|k|>n} |\Gamma_{rs}(k)|\right]\\
&= \frac{1}{2\pi}\left(\frac{\Omega_n(f_X)}{n} + L_n(f_X)\right).
\end{aligned}
\end{equation}
Noticing $|e^{ix} - e^{iy}|\le \sqrt{2} |x-y|$ and $|\omega_j-\omega_q| = 2\pi \frac{|j-q|}{n}$, 
\begin{equation}
\label{eq:mul_dev2}
\begin{aligned}
&\left|\frac{1}{2\pi} e_r^\top \left[\mathbb{E} I(\omega_j) - \mathbb{E} I(\omega_q) \right]e_s\right| \\
&= \frac{1}{2\pi}\left|\sum_{|k|\le n} \left(1-\frac{k}{n}\right) |\Gamma_{rs}(k)| (e^{-i\omega_jk} - e^{-i\omega_qk})\right|\\
&\le \frac{1}{2\pi} \sum_{|k|\le n} \sqrt{2} |\Gamma_{rs}(k)| |k||\omega_j - \omega_q| \\
&= \sqrt{2} |j-q| \frac{\Omega_n(f_X)}{n}. 
\end{aligned}
\end{equation}
Plug \eqref{eq:mul_dev1} and \eqref{eq:mul_dev2} and into \eqref{eq:mul_dev},  
\begin{equation}
\begin{aligned}
&\left|e_r^\top \left[\mathbb{E}\hat{f}(\omega_j) - f(\omega_j)\right]e_s\right| \le \frac{1}{2\pi}\left(\frac{\Omega_n(f_X)}{n} + L_n(f_X)\right)\\
&+\sqrt{2} \left(\frac{\sum_{|\ell|\le m} |\ell|}{2m+1}\right)\frac{\Omega_n(f_X)}{n}\\
&\le \frac{m}{n}\Omega_n(f_X) + \frac{1}{2\pi}\left(\frac{\Omega_n(f_X)}{n}+L_n(f_X)\right).
\end{aligned}
\end{equation}
\end{proof}

\subsection{Proof for Proposition \ref{prop:variance_bound}}
\begin{proof}
We focus on bounding the variance term
\begin{equation}
\mathbb{P}\left(\left|\hat{f}_{rs}(\omega_j) - \mathbb{E}\hat{f}_{rs}(\omega_j)\right| \ge \vertiii{f}\eta\right).
\end{equation}
% With the fact that for any $1\le r,s\le p$,
Since $\mathbb{P}\left(\left|\hat{f}_{rs}(\omega) - \mathbb{E}\hat{f}_{rs}(\omega)\right|\ge  \vertiii{f}\eta \right)$ is at most 
\begin{equation}
\label{eq:bound_with_real_img}
\begin{aligned}
&\mathbb{P}\left(\left|\hat{f}_{rs}(\omega) - \mathbb{E}\hat{f}_{rs}(\omega)\right|\ge  \vertiii{f}\eta \right) \\
&\le \mathbb{P}\left(\left|\mathbf{Re}\left(\hat{f}_{rs}(\omega) - \mathbb{E}\hat{f}_{rs}(\omega)\right)\right|\ge \frac{\vertiii{f}\eta}{2} \right) \\
& + \mathbb{P}\left(\left|\mathbf{Im}\left(\hat{f}_{rs}(\omega) - \mathbb{E}\hat{f}_{rs}(\omega)\right)\right|\ge \frac{\vertiii{f}\eta}{2} \right),
\end{aligned}
\end{equation}
it is sufficient to derive can derive upper bounds for the real and imaginary parts separately.\par 
The main idea in our proof is to express the real and imaginary parts of $\hat{f}(\omega_j)$ as quadratic forms in $vec(\mathcal{X}^\top)$, and apply Lemma \ref{lemma: hason_bound_time_gauss}. 
First, we express the peridogram $I_n(\omega_j)$ in terms of  trigonometric series. 
As pointed out before, $I(\omega_j)$ defined in \eqref{eq:single_periodogram} could be written as 
\begin{equation}
\label{eq:realImaginaryParts}
\begin{aligned}
I(\omega_j) = & \left(\mathcal{X}^\top C_j-  \iu \mathcal{X}^\top S_j\right) \left(\mathcal{X}^\top C_j-\iu \mathcal{X}^\top S_j\right)^\dag \\
= & \mathcal{X}^\top (C_jC_j^\top + S_jS_j^\top)\mathcal{X} + \iu \mathcal{X}^\top(C_jS_j^\top-S_jC_j^\top)\mathcal{X}.
\end{aligned}
\end{equation}
Now, \eqref{eq:realImaginaryParts} indicates that in the univariate case ($p=1$) the imaginary part becomes zero and we only need to bound the real part. However, for multivariate case, we need to understand the concentration behaviour of both parts. \par 
We will show the proof for imaginary part here and defer the proof for real part to  the appendix. \par  
We claim that 
for given unit vectors $u$ and $v$, there exists a universal positive constant $c$ such that for any $\eta > 0$,
\begin{equation}
\begin{aligned}
& \mathbb{P}\left(\left|u^\top \mathrm{\bf{Im}}\left(\hat{f}(\omega_j) - \mathbb{E}\hat{f}(\omega_j)\right)v\right|\ge 2\vertiii{f}\eta \right) \\
& \le 4\exp \left( - c\min \left((2m+1)\eta^2,(2m+1)\eta \right) \right).
\end{aligned}
\end{equation}
%\begin{proof}
To prove this claim, note that \eqref{eq:realImaginaryParts} implies
\begin{equation}
\mathrm{\bf{Im}}\left(\hat{f}(\omega_j)\right) = \mathcal{X}^\top\sum_{|\ell|\le m}(S_{j+\ell}C_{j+\ell}^\top - C_{j+\ell}S_{j+\ell}^\top)\mathcal{X} .
\end{equation}
Therefore,  
\begin{equation}
\label{eq:mul_im_two}
\begin{aligned}
&\mathbb{P}\left(\left|u^\top \mathrm{\bf{Im}}\left(\hat{f}(\omega_j) - \mathbb{E}\hat{f}(\omega_j)\right)v\right|\ge 2\vertiii{f} \eta \right) \le \\
&\mathbb{P}\left(\frac{1}{2\pi(2m+1)}\left|u^\top \mathcal{X}^\top\sum_{|\ell|\le m}(S_{j+\ell}C_{j+\ell}^\top)\mathcal{X}  v - \mathbb{E}\left\{u^\top \mathcal{X}^\top\sum_{|\ell|\le m}(S_{j+\ell}C_{j+\ell}^\top)\mathcal{X}  v\right\}\right|\ge \vertiii{f} \eta \right) \\
&+\mathbb{P}\left(\frac{1}{2\pi(2m+1)}\left|u^\top \mathcal{X}^\top\sum_{|\ell|\le m}(C_{j+\ell}S_{j+\ell}^\top)\mathcal{X}  v - \mathbb{E}\left\{ u^\top \mathcal{X}^\top\sum_{|\ell|\le m}(C_{j+\ell}S_{j+\ell}^\top)\mathcal{X}  v\right\}\right|\ge \vertiii{f} \eta \right).
\end{aligned}
\end{equation}
It takes the same technique to get upper bound for two parts in the second line in equation \eqref{eq:mul_im_two}. So we will only show the proof for getting upper bound for the first part. \par 
Let $Y_t = [v^\top ; u^\top ]X_t$ be a 2-dimensional time series. It follows from lemma \ref{lemma:max-L2-norm-Y} that $\vertiii{f_Y}\le \|[v^\top; u^\top]\|^2 \vertiii{f} = 2\vertiii{f}$. \par 
Define
\begin{equation}
P_j = \left[ 
\begin{array}{ll}
M_j & 0 \\
0 & N_j 
\end{array}
\right]_{(4m+2)\times{2n}}, 
\end{equation}
where 
\begin{align}
M_j=\begin{bmatrix}
S_{j-m}^\top\\
\vdots \\
S_j^\top\\
\vdots \\
S_{j+m}^\top
\end{bmatrix}_{(2m+1)\times n}  \qquad
N_j =\begin{bmatrix}
C_{j-m}^\top\\
\vdots \\
C_j^\top\\
\vdots \\
C_{j+m}^\top
\end{bmatrix}_{(2m+1)\times n}.
\end{align}
We can express the first part in \eqref{eq:mul_im_two} as 

\begin{equation}
\label{eq:mul_img_final}
\begin{aligned}
&\mathbb{P}\left(\frac{1}{2\pi(2m+1)}\left|u^\top \mathcal{\mathcal{X}}^\top\sum_{|\ell|\le m}(S_{j+\ell}C_{j+\ell}^\top)\mathcal{\mathcal{X}}  v - \mathbb{E}\left\{u^\top \mathcal{X}^\top\sum_{|\ell|\le m}(S_{j+\ell}C_{j+\ell}^\top)\mathcal{X}  v\right\}\right|\ge \vertiii{f} \eta \right)\\
& = \mathbb{P}\left(\frac{1}{2\pi(2m+1)}\left|vec(\mathcal{Y}^\top)^\top P_j^\top MP_j vec(\mathcal{Y}^\top)\ - \mathbb{E} \left\{vec(\mathcal{Y}^\top)^\top P_j^\top MP_j vec(\mathcal{Y}^\top)\right\}\right|\ge \vertiii{f}\eta\right), 
\end{aligned}
\end{equation}
where 
\begin{equation}
M = \left[
\begin{array}{ll}
0_{2m+1,2m+1} & I_{2m+1,2m+1}\\
0_{2m+1,2m+1} & 0_{2m+1,2m+1}
\end{array}
\right]. 
\end{equation}
Since $M_j$ and $N_j$ are both composed with rows from $Q_{F_n}$, $\|M_j\|\le \|Q_{F_n}\|=1$ and $\|N_j\|\le \|Q_{F_n}\|=1$. Furthermore, as block-wise diagonal matrix, $\|P_j\|=\max\{\|M_j\|, \|N_j\|\}=1$. 
Now $\|P_j^\top M P_j\|\le \|P_j\|^2\|M\| \le 1$ and $\rank(P_j^\top M P_j) \le \rank(M) = 2m+1$. Since $\vertiii{f_Y}\le 2\vertiii{f}$, we can apply lemma \ref{lemma: hason_bound_time_gauss} to show that the probability in \eqref{eq:mul_img_final} is at most 
\begin{equation}
\begin{aligned}
&2\exp\left(-c\min\left(\cfrac{(2m+1)\eta}{\|P_jMP_j^\top\|}, \cfrac{(2m+1)^2\eta^2}{\rank(P_j)\|P_jMP_j^\top\|}\right)\right) \\
&\le 2\exp\left(-c\min\left((2m+1)\eta, \cfrac{(2m+1)^2\eta^2}{(4m+2)}\right)\right) \\
& \le 2\exp\left(-c\min\left((2m+1)\eta^2, (2m+1)\eta\right)\right),
\end{aligned}
\end{equation}
where $c$ is an universal constant. 
%\end{proof}

A similar argument in Lemma \ref{lemma:mul_real} shows that the real part in \eqref{eq:realImaginaryParts} can be upper bounded as 
\begin{eqnarray}
\mathbb{P}\left(\left|u^\top \mathrm{\bf{Re}}\left(\hat{f}(\omega_j) - \mathbb{E}\hat{f}(\omega_j)\right)v\right|\ge 2 \vertiii{f} \eta \right) \nonumber \\
\le 6\exp \left( - c\min \left((2m+1)\eta^2,(2m+1)\eta \right) \right).
\end{eqnarray}

Combining the two bounds for real and imaginary parts, and plugging these two bounds in  \eqref{eq:bound_with_real_img}, we can show that there exist universal positive constants $c_1, c_2$ such that for any $\eta > 0$, 
\begin{equation}\label{eqn:conc-entrywise}
\mathbb{P}\left(\left|\hat{f}_{rs}(\omega_j) - \mathbb{E}\hat{f}_{rs}(\omega_j)\right| \ge \vertiii{f}\eta\right)\le c_1\exp\left(-c_2(2m+1)\min(\eta, \eta^2)\right).
\end{equation}
Setting $\eta = \sqrt{\frac{\log p}{m}}$ and combining with   \eqref{eq:change_bound_to_variance}, we have {\color{red} [drop $o(1)$]} 
\begin{equation}
  \mathbb{P}(\max_{r, s}|\hat{f}_{rs}(\omega_j)-f_{rs}(\omega_j)|\ge \tilde{\eta}) \le c_1 p^2\exp\left(-c_2 (2m+1)\frac{\log p}{m}\right).
\end{equation}
This concentration inequality proves the single deviation bound used in the proof of Theorem 1 as equation (12) in \citet{bickel2008covariance}. Then follow the technique of the proof in Theorem 1, we could get $L_1$ norm bound for error term in \eqref{eq:L1_error} and complete the proof.
\end{proof}
%\end{prop}

\subsection{Proof for Lemma \ref{lemma:heavy_tail_hanson}}
\begin{proof}
Proof for case \eqref{CA1} is given by \cite{rudelson2013hanson} and proof for case \eqref{CA2} is given by Lemma 8.3 in \cite{erdHos2012bulk}. We will show the proof for case \eqref{CA3} based on Markov inequality. We will show tail bound for both 
diagonal part and non-diagonal part for any $\eta \ge 0$ one by one. For diagonal part,  let $y_i = \varepsilon^2_{ii}-1$, then 
$\mathbb{E}y_i = 0$ and $\mathbb{E}y^2_i = \mathbb{E}\varepsilon^4_{ii} - 2\mathbb{E}\varepsilon^2_{ii}+1 =  K-1\le K$, therefore, noticing $\mathbb{E}\varepsilon'A\varepsilon = \text{tr}(A)$ under this setting, 

\begin{equation}
\begin{aligned}
&\mathbb{P}\left[\left|\sum_{i=1}^n \varepsilon^2_{ii} A_{ii} - \text{tr}(A)\right|\ge \eta\right] = \mathbb{P}\left[\left|\sum_{i=1}^n y_iA_{ii}\right|\ge \eta\right]\\
&\le \frac{\mathbb{E}(\sum_{i=1}^n y_iA_{ii})^2}{\eta^2} \le \frac{K\sum_{i=1}^n A^2_{ii}}{\eta^2}, 
\end{aligned}
\end{equation}
where the second last inequality is given by $\mathbb{E} y_iy_j = 0$. 
For the non diagonal part, note that
\begin{equation}
\begin{aligned}
&\mathbb{P}\left[\left|\sum_{1\le i<j\le n} A_{ij}\varepsilon_i\varepsilon_j \right|\ge \eta\right] \le \frac{\mathbb{E}\left|\sum_{1\le i< j\le n} A_{ij}\varepsilon_i\varepsilon_j \right|^2}{\eta^2} \\
& = \frac{\sum_{1\le i \neq j\le n} A^2_{ij}(\mathbb{E}\varepsilon^2_1)^2}{\eta^2} =  \frac{2\sum_{1\le i\neq j\le n} A^2_{ij}}{\eta^2},
\end{aligned}
\end{equation}
where the second line is given by $\mathbb{E}\varepsilon_i\varepsilon_j\varepsilon_p\varepsilon_q\neq 0$ iff $i=p,j=q$ or $i=q, i=p$. \par 
Then combining these two parts, we get
\begin{equation}
\begin{aligned}
    &\mathbb{P}\left[|\varepsilon^\top A\varepsilon - \mathbb{E} \varepsilon^\top A\varepsilon|\ge \eta\right] \\
    \leq& \mathbb{P}\left[\left|\sum_{i=1}^n \varepsilon ^2_{ii} A_{ii} - \text{tr}(A)\right|\ge \eta/2\right]+\mathbb{P}\left[\left|\sum_{1\le i<j\le n} A_{ij}\varepsilon_i\varepsilon_j \right|\ge \eta/2\right]\\
    \leq& \max\{4K,8\} \frac{\|A\|_F^2}{\eta^2},
\end{aligned}
\end{equation}
where we could set $c=\max\{4K,8\}$ to complete our proof. 
\end{proof}
