# Supplementary material for: Large Spectral Density Matrix Estimation by Thresholding
Source: arXiv:1812.00532 source file (2018-12-03)
Supplement: Supplementary file 3 [file appendix_simulation_setting.tex]

\section{More on Simulation Setting}
\label{sec:simulation_setting}

\begin{figure}[H] 
\centering 
    \begin{minipage}{.2\textwidth}
    \includegraphics[scale = 0.15]{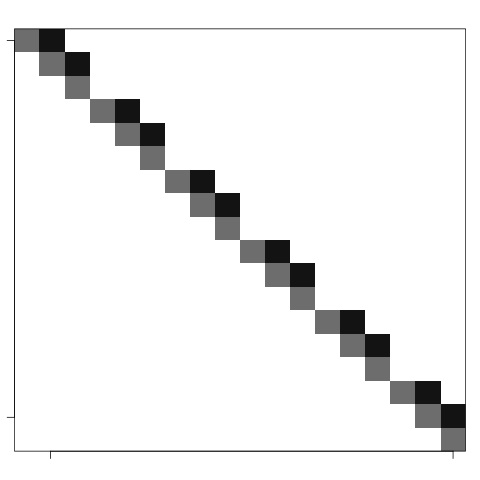}
    \end{minipage}
    \begin{minipage}{.2\textwidth}
    \includegraphics[scale = 0.15]{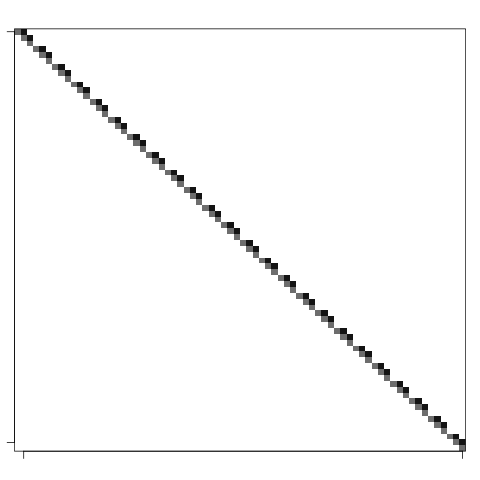}
    \end{minipage} 
     \begin{minipage}{.2\textwidth}
    \includegraphics[scale = 0.15]{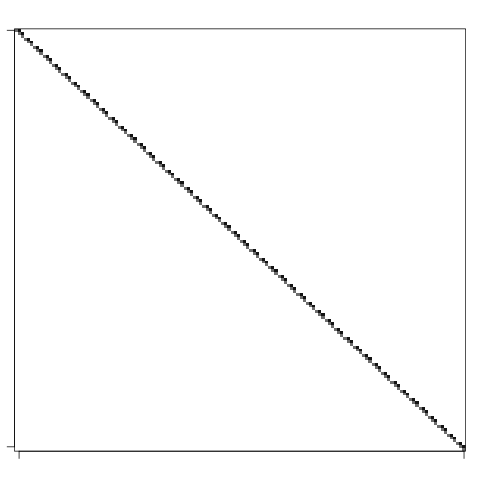}
    \end{minipage} \\
\caption{Element-wise absolute value of transition matrix $A$ and $B$ for $p = 12, 48, 96$ in the homogeneous setting for VAR(1) in simulation studies}
\label{fig::Ahomo}
\end{figure}

\newpage
