# Supplementary material for: Large Spectral Density Matrix Estimation by Thresholding
Source: arXiv:1812.00532 source file (2018-12-03)
Supplement: Supplementary file 4 [file appendix_tech_proof.tex]

\section{Appendix: Proof of Technical Results}
\label{sec:proof_for_technical_lemmas}

\begin{lem}
\label{lemma:q_norm_eq}
For any matrix $A\in \mathbb{C}^{p \times p}$ and  $0<q<1$, define $\|A\|_q:= $ {\color{red} [re-define]}. Then 
\begin{equation}
\max_{s=1}^p  \sum_{r=1}^p |A_{rs}|^q = \|A\|_q^q.
\end{equation}
\begin{proof}
First, for two vectors $v_1, v_2\in \mathbb{C}^p$, $\|v_1+v_2\|_q^q\le \|v_1\|_q^q + \|v_2\|_q^q$ for $0<q<1$, since for scalars $x,y\in \mathbb{C}$, $|x+y|^q \le |x|^q+|y|^q$. Then let $A_i$ be the $i^{th}$ column of $A$. Based on the definition of $\|A\|_q$, 
\begin{equation}
\begin{aligned}
& \|A\|_q^q = \max_{\|x\|_q = 1} \|\sum_{i=1}^p A_ix_i\|_q^q \\
& \le  \max_{\|x\|_q = 1} \sum_{i=1}^p \|A_ix_i\|_q^q  = \sum_{i=1}^p |x_i|^q\|A_i\|_q^q\\
&\le (\max_{i=1}^p \|A_i\|_q^q) \sum_{i=1}^p\|x_i\|^q = \max_{i=1}^p \|A_i\|_q^q,
\end{aligned}
\end{equation}
which finishes the proof. 
\end{proof}
\end{lem}

\begin{lem}
\label{lemma:spectral_simple}
For any matrix $M\in \mathbb{R}^{p\times p}$, and a positive constant $\epsilon$, we could add a matrix $E$ such that $A+E$ has distinct eigenvalues and $\|E\|\le \epsilon$. 
\begin{proof}
Consider the Schur decomposition(\citep{golub2012matrix}) of $M$ as $M=QUQ^\dag$ where $Q$ is an unitary matrix and $U$ is an upper triangular matrix. Construct a digonal matrix
$D$ with each element less than $\epsilon$ and make $U_{i,i} + D_{i,i}$ distinct. Set $E = QDQ^\dag$, we have $A+QDQ^\dag = Q (E+D)Q^\dag$ with eigenvalues as $U_{i,i} + D_{i,i}, i=1,\dots p$ which are distinct. By setting $E= QDQ^\dag$ and noticing $\|E\| = \|QDQ^\dag\| = \|D\|\le \epsilon$ we complete the proof. 
\end{proof}
\begin{remark}
$|\Lambda_{\text{max}}(A)|$ is continuous mapping from matrix to real number, thus, we could always find perturbation $\|E\|$ small enough to guarantee $\|A+E\|<1$. To quantify this, we may apply result for \citet{bhatia1990bounds} for perturbation bound for general matric which may not be symmetric:
\begin{equation}
\label{eq:eigen_bound}
|\rho(A+E)-\rho(A)|\le 12\|A\|^{1-1/n}\|E\|^{1/n}.
\end{equation}
\end{remark}
\end{lem}

For VAR(1) defined in \eqref{eqn:var_dto1}, if $\tilde{A}$ is diagonalizable, i.e., it could be written as $\tilde{A}=SDS^{-1}$ where 
$S$ is the matrix formed with its eigen-vectors and $D$ is the digonal matrix, then
\begin{equation}
\Omega_n(f) \le 2\kappa(p)\frac{\rho(\tilde{A}_1)}{(1-\rho(\tilde{A}_1))^3}, 
\end{equation}
where $\kappa(p) = \|S^{-1}\|\|S\|$.
\begin{proof}

%%%%%%%%%%%%%%%%%%%%%%%%%%%%%%%
% Pf: bounding bias
%%%%%%%%%%%%%%%%%%%%%%%%%%%%%%%
\subsection*{Proof for proposition \ref{prop:bias_bound}}
\begin{proof}
It suffices to show that for any unit vector $v,u$, 
\begin{equation}
\begin{aligned}
\left|v^\top \left[\mathbb{E}\hat{f}(\omega_j) - f(\omega_j)\right]u\right| \le \frac{m}{n}\Omega_n(f) + \frac{1}{2\pi}\left(\frac{\Omega_n(f)}{n}+L_n(f)\right). 
\end{aligned}
\end{equation}
Recall 
\begin{equation}
\hat{f}(\omega_j) = \frac{1}{2\pi}\frac{1}{2m+1} \sum_{\ell =-m}^m I(\omega_{j+\ell}), 
\end{equation}
we could have 
\begin{equation}
\label{eq:mul_dev}
\begin{aligned}
\left|v^\top \left[\mathbb{E}\hat{f}(\omega_j) - f(\omega_j)\right]u\right| 
&\le \left|v^\top \left[\frac{1}{2\pi}\mathbb{E}I(\omega_j) - f(\omega_j)\right]u\right|\\
&+\frac{1}{2\pi(2m+1)} \sum_{\ell = -m}^m |v^\top\left[\mathbb{E}I(\omega_{j+\ell}) - I(\omega_{j})\right]u|.
\end{aligned}
\end{equation}
With definition of $I_n(\omega_j)$ in \eqref{eq:single_periodogram}, we have 
\begin{equation}
\label{eq:mul_dev1}
\begin{aligned}
\left|\frac{1}{2\pi} v^\top \left[\mathbb{E} I(\omega_j) - 2\pi f(\omega_j)\right]u\right| &= \frac{1}{2\pi}\left|\sum_{|k|\le n} \frac{k}{n}  (v^\top \Gamma(k)u) e^{-i\omega_j k}+\sum_{|k|>n} (v^\top \Gamma(k)u) e^{-i\omega_jk}\right|\\
&\le \frac{1}{2\pi} \left [\sum_{|k|\le n} \frac{k}{n}  \|\Gamma(k)\|+ \sum_{|k|>n}\|\Gamma(k)\|\right]\\
&= \frac{1}{2\pi}\left(\frac{\Omega_n(f)}{n} + L_n(f)\right).
\end{aligned}
\end{equation}
Noticing $|e^{ix} - e^{iy}|\le \sqrt{2} |x-y|$ and $|\omega_j-\omega_q| = 2\pi \frac{|j-q|}{n}$, 
\begin{equation}
\label{eq:mul_dev2}
\begin{aligned}
&\left|\frac{1}{2\pi} v^\top \left[\mathbb{E} I(\omega_j) - \mathbb{E} I(\omega_q) \right]u\right| \\
&= \frac{1}{2\pi}\left|\sum_{|k|\le n} \left(1-\frac{k}{n}\right) (v^\top \Gamma(k)u) (e^{-i\omega_jk} - e^{-i\omega_qk})\right|\\
&\le \frac{1}{2\pi} \sum_{|k|\le n} \sqrt{2} \|\Gamma(k)\| |k||\omega_j - \omega_q| \\
&= \sqrt{2} |j-q| \frac{\Omega_n(f)}{n}. 
\end{aligned}
\end{equation}
Plug \eqref{eq:mul_dev1} and \eqref{eq:mul_dev2} and into \eqref{eq:mul_dev},  
\begin{equation}
\begin{aligned}
&\left|v^\top \left[\mathbb{E}\hat{f}(\omega_j) - f(\omega_j)\right]u\right| \le \frac{1}{2\pi}\left(\frac{\Omega_n(f)}{n} + L_n(f)\right)\\
&+\sqrt{2} \left(\frac{\sum_{|\ell|\le m} |\ell|}{2m+1}\right)\frac{\Omega_n(f)}{n}\\
&\le \frac{m}{n}\Omega_n(f) + \frac{1}{2\pi}\left(\frac{\Omega_n(f)}{n}+L_n(f)\right).
\end{aligned}
\end{equation}
\end{proof}

\begin{lem}
\label{lemma:orthogonal-cos-sin}
For any $j, k$ in $F$, the inner product between $C_j$, and $S_k$, can only have following forms:
\begin{enumerate}
\item[(a)] $C^{\top}_j S_k = 0$ for any $j$ and $k$ in $F_n$ 
\item[(b)] 
\begin{equation}
C_j^\top C_k = 
\begin{cases}
1 & \text{if}~ j=k=\frac{n}{2} ~\text{or}~ 0 \\
\frac{1}{2} & \text{if}~ j=k ~\text{or}~ j=-k\\
0 & \text{otherwise}
\end{cases}
\end{equation}
\item[(c)] \begin{equation}
S_j^\top S_k = 
\begin{cases}
\frac{1}{2} & \text{if}~ j=k ~\text{and}~ j\neq \frac{n}{2}  ~\text{and}~ j\neq 0 \\
-\frac{1}{2} & \text{if}~ j=-k\\
0 & \text{otherwise}
\end{cases}
\end{equation} 
\end{enumerate}
\begin{proof}
We first state Lagrange's trigonometric identities: 
\begin{equation}
\label{eq:cos_series}
\sum_{k=1}^n \cos(k\theta) = 
\begin{cases}
1 & \theta = 2k\pi ~\text{for some integer}~ k \\
-\frac{1}{2}+\frac{\sin\left(n+\frac{1}{2}\right)\theta}{2\sin \frac{\theta}{2}}  & \text{otherwise}
\end{cases}
\end{equation}
and 
\begin{equation}
\label{eq:sin_series}
\sum_{k=1}^n \sin(k\theta) =
\begin{cases}
0 & \theta = 2k\pi ~\text{for some integer}~ k \\ 
\frac{\cos \theta}{2\sin \theta}-\frac{\cos\left(n+\frac{1}{2}\right)\theta}{2\sin \frac{\theta}{2}} & \text{otherwise}
\end{cases}
\end{equation}
Now we consider a special case where we set $\mathbf{\theta} = \omega_j = \frac{2j\pi}{n}, j\in \mathbb{Z}$. Here we relax $j\in F_n$ to all integers. After this relaxation, we can write $\omega_j+\omega_k = \omega_{j+k}$ and $\omega_j-\omega_k = \omega_{j-k}$, using \eqref{eq:cos_series} and \eqref{eq:sin_series}.
For any $\omega_z$, $z\in \mathbb{Z}$, and fixed $n$, 

\begin{equation}
\label{eq:omega_cos}
\sum_{\ell=1}^n \cos(\ell\omega_z) = 
\begin{cases}
n & z\equiv 0\pmod{n} \\
-n & (z -\frac{n}{2}) \equiv 0\pmod{n} ~~n ~~\text{is even}\\
0  & \text{otherwise}
\end{cases}
\end{equation}

\begin{equation}
\label{eq:omega_sin}
\sum_{\ell=1}^n \sin(\ell\omega_z) = 0
\end{equation}

\par
Now we prove (a), (b) and (c).

\begin{enumerate}
\item[(a)] For any $j$ and $k$ in $F_n$, \eqref{eq:omega_sin} implies
\begin{equation}
\label{eq:case_a_proof}
C_j^\top S_k = \frac{1}{2n}\sum_{\ell=1}^n \sin\{\ell (\omega_j+\omega_k)\} = \frac{1}{2n}\sum_{\ell=1}^n \sin\{\ell (\omega_{j+k})\} = 0
\end{equation}
\item[(b)] For any $j,k\in F_n$, 
\begin{equation}
\label{eq:case_b_proof}
C_j^\top C_k = \frac{1}{2n}\left(\sum_{\ell=1}^n \cos \ell\omega_{j+k} + \sum_{\ell=1}^n \cos \ell\omega_{j-k}\right)
\end{equation}
For the case $j=k$, \eqref{eq:cos_series} implies
\begin{equation}
\label{eq:j=k_cos}
C_j^\top C_k = \frac{1}{2n} \left(\sum_{\ell=1}^n\cos \ell\omega_{n} + \sum_{\ell=1}^n \cos \ell\omega_{0}\right).
\end{equation}
If $j = \frac{n}{2}$ or $j=0$, $j+k\equiv 0 \pmod{n}$, which set \eqref{eq:j=k_cos} to be one. In other cases, it is straightforward that since $j,k\in F_n$, $-n<j+k<n$ and $j+k\neq 0$. Then \eqref{eq:case_b_proof} becomes $\frac{1}{2}$ with \eqref{eq:cos_series}. \par 
Then for the case $j=-k$, recall the definition of $F_n$. Note that $j$ and $k$ cannot be $\frac{n}{2}$ or $-\frac{n}{2}$ at the same time indicating $j-k \not \equiv 0 \pmod{n}$. Then with \eqref{eq:cos_series}, \eqref{eq:case_b_proof} becomes 
\begin{equation}
C_j^\top C_k = \frac{1}{2n}\left(\sum_{\ell=1}^n \cos \ell\omega_{0} + \sum_{\ell=1}^n \cos \ell\omega_{j-k}\right) = \frac{1}{2}
\end{equation}
For the other cases, $j+k\not \equiv 0 \pmod{n}$ and $j-k \not \equiv 0 \pmod{n}$, equation \eqref{eq:case_b_proof} becomes 0. 
\item[(c)] for any $j,k\in F_n$, 
\begin{equation}
\label{eq:case_c_proof}
C_j^\top C_k + S_j^\top S_k = \frac{1}{n}\sum_{\ell=1}^n \cos \ell\omega_j \cos \ell\omega_k + \sin \ell\omega_j\sin \ell\omega_k = \frac{1}{n}\sum_{\ell=1}^n \cos (\ell\omega_{j-k})
\end{equation}
If $j=k$, \eqref{eq:case_c_proof} becomes 1. If $j\neq k$, $-n<j-k<n$ and $j-k\neq 0$ indicating $j-k\not \equiv 0 \pmod{n}$, so \eqref{eq:case_c_proof} becomes 0. Plugging in the value in (b) into this \eqref{eq:case_c_proof}, complete the proof for (c). 
\end{enumerate}
\end{proof}
\end{lem}

\begin{lem}
\label{lemma:maximum_L2_Q}
$\|Q_{F_n}\|= 1$
where 
\begin{equation}
Q_{F_n} = \begin{bmatrix}
C_{-[\frac{n-1}{2}]}^\top\\ 
S_{-[\frac{n-1}{2}]}^\top \\
\vdots \\
C_{[\frac{n}{2}]}^\top\\ 
S_{[\frac{n}{2}]}^\top \\
\end{bmatrix}
\end{equation}
and each $C_j, S_j, j\in F_n$ follow the definition in \eqref{eq:cos_sin_coef} 
\begin{proof}
Since row permutation does not change the $L_2$ norm of a matrix, we can stack rows in $Q_{F_n}$ such that $S_j,C_j,S_{-j}, C_{-j}$ appear adjacently, if there exists such a pair $\{j, -j\}$. Then $\|Q_{F_n}\|=\|Q^\top_{F_n}\| = \Lambda(Q_{F_n}Q_{F_n}^\top)$. Lemma \ref{lemma:orthogonal-cos-sin} implies that $Q_{F_n}Q_{F_n}^\top$ could only be block-wise diagonal with three possible blocks:
\begin{equation*}
B_1=\begin{bmatrix}
1&0\\
0&0
\end{bmatrix} ~~B_2 = \begin{bmatrix}
\frac{1}{2} & 0 & \frac{1}{2} & 0\\
0 & \frac{1}{2} & 0 & -\frac{1}{2}\\
\frac{1}{2} & 0 & \frac{1}{2} & 0 \\
0 & -\frac{1}{2} & 0 & \frac{1}{2}
\end{bmatrix}~~
B_3 = \begin{bmatrix}
\frac{1}{2} & 0\\
0 & \frac{1}{2}
\end{bmatrix}
\end{equation*}
This further follow that $\|Q_{F_n}\|=\Lambda_{\max}(Q_{F_n}Q_{F_n}^\top )\le \max_{i=1}^3 \|B_i\|=1$. We complete our proof. 
\end{proof}
\end{lem}

\begin{lem}
\label{lemma:max-L2-norm}
\[
2\pi \EuFrak{m}(f) \le \Lambda_{\text{min}}(\cov(vec(\mathcal{\mathcal{X}}^\top))) \le \Lambda_{\text{max}}(\cov(vec(\mathcal{\mathcal{X}}^\top)) \le 2\pi \mathcal{M}(f),
\]
where we follow the notation of $\mathcal{\mathcal{X}}$ and $\mathcal{M}(f)$ and $\EuFrak{m}(f)  = \essinf_{\omega \in [-\pi, \pi]}\|f(\omega)\|$. The lower bound we will not use in this paper, but for completeness of this lemma, we keep it there. 
\begin{proof}
The proof follows from Proposition 2.3 in \citet{Basu2015}. 
\end{proof}
\end{lem}

\begin{lem}
\label{lemma:max-L2-norm-Y}
For any matrix $A_{p\times m}$, the time series $Y_t = A^\top \mathcal{X}_t$ satisfies
\begin{equation}
\mathcal{M}(f_Y) \le \|A\|^2 \mathcal{M}(f).
\end{equation}
\begin{proof}
After transformation, $\mathcal{Y} = [\mathcal{X}_1^\top A; \dots; \mathcal{X}_n^\top A]$. The autocovariance for $Y_t$ can be written as 
\begin{equation}
    \Gamma_Y(\ell) = \cov(A^\top \mathcal{X}_t, A^\top \mathcal{X}_{t+\ell}) = A^\top \Gamma_\mathcal{X}(\ell) A,
\end{equation}
which immediately indicates that 
\begin{equation}
f_Y(\omega) = \sum_{\ell=-\infty}^\infty A^\top \Gamma_\mathcal{X}(\ell)A e^{-\iu\omega\ell} = A^\top  f(\omega)A.
\end{equation}
Thus for any $\omega \in [-\pi, \pi]$, $\|f_Y(\omega)\| \le \|A\|^2\mathcal{M}(f)$. Taking supremum from both sides completes the proof. 
\end{proof}
\end{lem}

\begin{lem}
\label{lemma:linear_assumption}
For stationary infinite multivariate moving average, $\Gamma(\ell)$ is well defined, and assumption \ref{assumption:finite_auto} holds.
\begin{proof}
Since $(\sum_{i=1}^n |a_i|)^2 \ge \sum_{i=1}^n a_i^2$, 
\begin{equation}
\sum_{\ell=0}^\infty \|B_\ell\|_F \le \sum_{\ell=0}^\infty \sum_{1\le i,j\le p} |B_{\ell, (i,j)}|<\infty.
\end{equation}
Then by equivalence of norm, it follows that
\begin{equation}
\sum_{\ell=0}^\infty \|B_\ell\| < \infty.
\end{equation}
Therefore, 
\begin{equation}
\label{eq:finite_sum_auto}
\sum_{\ell = -\infty}^\infty \|\Gamma(\ell)\| = \sum_{\ell = -\infty}^\infty \|\sum_{t=0}^\infty B_t B_{t+\ell}^\top \|<
\sum_{\ell = -\infty}^\infty (\sum_{t=0}^\infty \|B_t\|)^2<\infty.
\end{equation}
\end{proof}
\end{lem}

\begin{lem}
\label{lemma:L2_convergence_truncate}
\begin{equation}
\lim_{L\rightarrow \infty}\mathbb{E} \left[ \|vec(\mathcal{\mathcal{X}}_{(L)}^\top) - vec(\mathcal{\mathcal{X}}^\top)\|^2 \right]  = 0,
\end{equation}
where $\mathcal{\mathcal{X}}_{n\times p} = [\mathcal{X}_1: \ldots : \mathcal{X}_n]^\top$ be the data matrix of a stationary linear forecast defined in \eqref{eq:infinite_ma}.
\begin{proof}
Since
\begin{equation}
\|vec(\mathcal{\mathcal{X}}_{(L)}^\top) - vec(\mathcal{\mathcal{X}}^\top)\|^2 = \sum_{t=1}^n \|\mathcal{X}_t-\mathcal{X}_{(L), t}\|^2,
\end{equation}
it suffices to show that $\lim_{L\rightarrow \infty}\mathbb{E} \left[ \|\mathcal{X}_{(L), t} - \mathcal{X}_t\|^2 \right] = 0$ for any given $t\in \{1,\dots, n\}$. It follows that 
\begin{equation}
\label{eq:dct_dominant}
\|\mathcal{X}_{(L), t}-\mathcal{X}_t\|^2 = \sum_{\ell_1=L+1}^\infty \sum_{\ell_2=L+1}^\infty \varepsilon_{t-{\ell_1}}^\top B^\top_{\ell_1} B_{\ell_2}\varepsilon_{t-{\ell_2}} \le \sum_{\ell_1=0}^\infty \sum_{\ell_2=0}^\infty\|B_{\ell_1}\|\|B_{\ell_2}\|\|\varepsilon_{t-{\ell_1}}\|
\|\varepsilon_{t-{\ell_1}}\|.
\end{equation}
Since $\varepsilon_t$ has finite second moment (1 actually), we let 
$\mathbb{E}\|\varepsilon_{t-{\ell_1}}\| = c_\varepsilon <\infty $. Then the expected value of right part in \eqref{eq:dct_dominant} is
\begin{equation}
c_\varepsilon^2 \sum_{\ell_1=0}^{\infty}\sum_{\ell_2=0}^{\infty} \|B_{\ell_1}\| \|B_{\ell_2}\| = c_\varepsilon^2(\sum_{\ell=0}^\infty \|B_{\ell}\|)^2<\infty, 
\end{equation}
where the last inequality was established in the proof of lemma \eqref{lemma:linear_assumption}. Then we apply dominated convergence theorem to show that 
\begin{equation}
\begin{aligned}
&\mathbb{E} \left[\|\mathcal{X}_{(L), t}-\mathcal{X}_t\|^2 \right] = \sum_{\ell_1=L+1}^\infty \sum_{\ell_2=L+1}^\infty \mathbb{E}\left[ \varepsilon_{t-{\ell_1}}^\top B^\top_{\ell_1} B_{\ell_2}\varepsilon_{t-{\ell_2}} \right]\\
& \sum_{\ell=L+1}^\infty \mathbb{E} \left[ \varepsilon_{t-\ell}^\top B^\top_{\ell_1} B_{\ell_2} \varepsilon_{t-\ell} \right] \le c_\varepsilon^2 (\sum_{\ell=L+1}^\infty \|B_\ell\|)^2,
\end{aligned}
\end{equation}
because $\sum_{\ell=0}^\infty \|B_\ell\|<\infty$, above goes to zero when $L\rightarrow \infty$. 
\end{proof}
\end{lem}
\begin{remark}
We could immediately get several results:
\begin{enumerate}
    \item $vec(\mathcal{\mathcal{X}}_{(L)}^\top)\overset{\mathbb{P}}{\to} vec(\mathcal{\mathcal{X}}^\top)$
    \item Given any given matrix $A_{np\times np}$,
    \begin{equation}
       \lim_{L\rightarrow \infty}\mathbb{E} \left[ vec(\mathcal{\mathcal{X}}_{(L)}^\top)^\top A ~ vec(\mathcal{\mathcal{X}}_{(L)}}^\top)\right] =  \lim_{L\rightarrow \infty}\mathbb{E} \left[ vec(\mathcal{\mathcal{X}}^\top)^\top A ~ vec(\mathcal{\mathcal{X}}^\top)\right]
    \end{equation}
This is because
\begin{equation}
\label{eq:cross_terms_bound}
\begin{aligned}
&\left|\mathbb{E} \left[ vec(\mathcal{\mathcal{X}}_{(L)}^\top)^\top A ~ vec(\mathcal{\mathcal{X}}_{(L)}}^\top)\right] - \mathbb{E} \left[ vec(\mathcal{\mathcal{X}}^\top)^\top A ~ vec(\mathcal{\mathcal{X}}^\top)\right]\right| \\
&\left|\mathbb{E} \left[ vec(\mathcal{\mathcal{X}}_{(L)}^\top)^\top A  \left(vec(\mathcal{\mathcal{X}}_{(L)}}^\top)-vec(\mathcal{\mathcal{X}}^\top)\right)\right]\right|+\left|\left(vec(\mathcal{\mathcal{X}}_{(L)}}^\top)-vec(\mathcal{\mathcal{X}}^\top)\right)^\top A ~ vec(\mathcal{\mathcal{X}}^\top )\right|.
\end{aligned}
\end{equation}
Apply cauchy inequality to the first part in second line of \eqref{eq:cross_terms_bound}
\begin{equation}
\begin{aligned}
&\left|\mathbb{E} \left[ vec(\mathcal{\mathcal{X}}_{(L)}^\top)^\top A  \left(vec(\mathcal{\mathcal{X}}_{(L)}}^\top)-vec(\mathcal{\mathcal{X}}^\top)\right)\right]\right|^2 \\
&\le \|A\| \mathbb{E} \left[ \|vec(\mathcal{\mathcal{X}}_{(L)}^\top)\|^2\right] \mathbb{E} \left[ \left\|\left(vec(\mathcal{\mathcal{X}}_{(L)}}^\top)-vec(\mathcal{\mathcal{X}}^\top)\right)\right\|^2\right].
\end{aligned}
\end{equation}
But from lemma \eqref{lemma:L2_convergence_truncate}, 
$\mathbb{E} \left[ \|vec(\mathcal{\mathcal{X}}_{(L)}^\top)\|^2\right]\right]\rightarrow \mathbb{E} \left[ \|vec(\mathcal{\mathcal{X}}^\top)\|^2\right]\right] $ and \\
 $ \mathbb{E} \left[ \|\left(vec(\mathcal{\mathcal{X}}_{(L)}}\top)-vec(\mathcal{\mathcal{X}}^\top)\right)\|^2\right]\rightarrow 0$ indicating first part in second line of \eqref{eq:cross_terms_bound} convergences to zero when $L$ goes to infinity. Similarly, we could also show the second part in second line of \eqref{eq:cross_terms_bound} goes to zero too. Then we finish our proof.
\end{enumerate}
\end{remark}

\begin{lem}
\label{lemma:spectral_convergence}
$\lim_{L\rightarrow \infty}\vertiii{f_{(L)}} = \vertiii{f}$.
\begin{proof}
Let $\Gamma_{(L)}(h)$ and $f_{(L)}(\omega)$ be the autocovariance and spectral density for truncated process $X_{(L)}$ respectively. Then for any frequency $\omega \in [-\pi, \pi]$,
\begin{equation}
\label{eq: bound_by_autocovariance}
\|f_{(L)}(\omega)-f(\omega)\| \le \sum_{h=-\infty}^\infty \|\Gamma_{(L)}(h)-\Gamma(h)\|\|e^{-\iu \omega h}\|= \sum_{h=-\infty}^\infty \|\Gamma_{(L)}(h)-\Gamma(h)\|.
\end{equation}
for any $h\in \mathbb{Z}$, without loss of generality, we will show that when $h\geq 0$, we have
\begin{equation}
    \Gamma_{(L)}(h) = \sum_{\ell=0}^{L-h} B_\ell B_{\ell+h}^\top.
\end{equation}
Then for any given $h\in \mathbb{Z}^+$, 
\begin{equation}
\begin{aligned}
\lim_{L\rightarrow \infty}\|\Gamma_{(L)}(h) - \Gamma(h)\|& = \lim_{L\rightarrow \infty} \left\|\sum_{\ell= L - h +1}^\infty B_\ell B_{\ell+h}^\top \right\| \\ 
&\le \lim_{L\rightarrow \infty}\sum_{\ell=L-h+1}^\infty \|B_\ell\|  \|B_{\ell+h}\|\\ 
&\le \lim_{L\rightarrow \infty} \left(\sum_{\ell=0}^\infty \|B_{\ell}\|\right) \left(\sum_{\ell=L+1}^\infty \|B_{\ell}\|\right)  =0.
\end{aligned}
\end{equation}
The last equality comes from the fact that $\sum_{\ell=0}^\infty \|B_\ell\|<\infty$. 
It follows that 
\begin{equation}
\begin{aligned}
\max\left\{\sum_{h=-\infty}^\infty \|\Gamma(h)\|, \sum_{h=-\infty}^\infty\|\Gamma_{(L)}(h)\|\right\}\le (\sum_{\ell=-\infty}^\infty \|B_\ell\|)^2<\infty,
\end{aligned}
\end{equation}
which in turn implies 
\begin{equation}
\label{eq:autocovariance_dct}
\sum_{h=-\infty}^\infty \|\Gamma_{(L)}(h) - \Gamma(h)\| \le (\sum_{\ell=-\infty}^\infty \|B_\ell\|)^2<\infty.
\end{equation}
Therefore, 
\begin{equation}
\begin{aligned}
&\lim_{L\rightarrow \infty}\sup_{\omega\in [-\pi, \pi]}\|f_{(L)}(\omega)-f(\omega)\|\le \lim_{L\rightarrow \infty}\sum_{h=-\infty}^\infty \|\Gamma_{(L)}(h)-\Gamma(h)\|\\
& = \sum_{h=-\infty}^\infty  \lim_{L\rightarrow \infty}  \|\Gamma_{(L)}(h)-\Gamma(h)\| = 0,
\end{aligned}
\end{equation}
where the second line is obtained from applying dominated convergence theorem to counting measure where dominated convergence theorem is guaranteed to be used with \eqref{eq:autocovariance_dct}. Finally
\begin{equation}
\begin{aligned}
&\lim_{L\rightarrow \infty}\left|\vertiii{f_{(L)}} - \vertiii{f}\right| =\lim_{L\rightarrow \infty} \left|\sup_{\omega\in [-\pi, \pi] }\|f_{(L)}(\omega)\|-\sup_{\omega\in [-\pi, \pi] }\|f(\omega)\| \right|\\
&\le \lim_{L\rightarrow \infty} \esssup_{\omega \in [-\pi, \pi]}\|f_{(L)}(\omega)-f(\omega)\| =0, 
\end{aligned}
\end{equation}
which completes the proof.  
\end{proof}
\end{lem}
